# Supplementary material for: LoneSTAR: Analog Beamforming Codebooks for Full-Duplex Millimeter Wave Systems
Source: arXiv:2206.11418 source file (2022-06-22)
Supplement: Supplementary file 1 [file sec-appendix.tex]

\appendices

\section{Test}
